# Supplementary material for: Expecting The Unexpected: Towards Broad Out-Of-Distribution Detection
Source: arXiv:2308.11480 source file (2024-12-09)
Supplement: Supplementary file 1 [file dataset_info.tex]

\textbf{Github repo with script to acquire BROAD splits:} \url{https://github.com/ServiceNow/broad}

\textbf{Huggingface dataset card:} \url{https://huggingface.co/datasets/ServiceNow/PartialBROAD}

\textbf{License:} This work is licensed under a Creative Commons Attribution 4.0 Unported License.
